# Supplementary material for: Distributed Rate-Splitting Multiple Access for Multilayer Satellite Communications
Source: arXiv:2307.07382 source file (2024-05-02)
Supplement: Supplementary file 2 [file Appendix.tex]

% Appendix
\begin{appendices}
	\section{Signal Power Segments}\label{Append:sign_power}
	The power segments of common stream received at \gls{geo} \gls{gu}-$n$ is
	\begin{subequations}
		\begin{align}
			 & A_{g,cn}=S_{g,cn}^\prime+S_{g,pn}^\prime+{I_{g,n}^{tot}}^\prime+\sigma_n^2, \\
			 & B_{g,cn}=S_{g,pn}^\prime+{I_{g,n}^{tot}}^\prime+\sigma_n^2,
		\end{align}
	\end{subequations}
	where $S_{g,cn}^\prime=\tr\left(\mathbf{H}_{g,n}\mathbf{F}_{g,c}\right)$.
	\par For \gls{leo} \gls{lu}-$k_m$, the power segments of decoding the common stream transmitted from \gls{geo} is expressed as
	\begin{subequations}
		\begin{align}
			 & A_{supc,k_m}=S_{g2l,ck_m}^\prime+S_{l,ck_m}^\prime+S_{l,pk_m}^\prime+{I_{l,k_m}^{tot}}^\prime+\sigma_n^2, \\
			 & B_{supc,k_m}=S_{l,ck_m}^\prime+S_{l,pk_m}^\prime+{I_{l,k_m}^{tot}}^\prime+\sigma_n^2,
		\end{align}
	\end{subequations}
	where $S_{g2l,ck_m}^\prime$, $S_{l,ck_m}^\prime$,$S_{l,pk_m}^\prime$,$I_{il,pk_m}^\prime$,$I_{gl,k_m}^\prime$ can be further expressed as
	\begin{subequations}
		\begin{align}
			 & S_{g2l,ck_m}^\prime=\tr\left(\mathbf{H}_{g2l,k_m}\mathbf{F}_{g,c}\right),                   \\
			 & S_{l,ck_m}^\prime=\tr\left(\mathbf{H}_{l,mk_m}\mathbf{F}_{l,cm}\right),                     \\
			 & S_{l,pk_m}^\prime=\tr\left(\mathbf{H}_{l,mk_m}\mathbf{F}_{l,pk_m}\right),                   \\
			 & I_{il,pk_m}^\prime=\sum_{\substack{i=1,                                                     \\i\neq k_m}}^{K_m}\tr\left(\mathbf{H}_{l,mk_m}\mathbf{F}_{l,pi}\right),                                                                                                                                           \\
			 & I_{gl,k_m}^\prime=\tr\left(\mathbf{H}_{g2l,k_m}\mathbf{F}_{g,p}\right)+\sum_{\substack{j=1, \\j\neq m}}^{M}\tr\left(\mathbf{H}_{l,jk_m}\mathbf{F}_{l,pj}\right) \\
			 & \quad\quad\quad+\sum_{\substack{j=1,                                                        \\j\neq m}}^{M}\sum_{i=1}^{K_j}\tr\left(\mathbf{H}_{l,jk_m}\mathbf{F}_{l,pi}\right).
		\end{align}
	\end{subequations}
	The power segments of decoding sub-common stream, $s_{subc,m}$, and private stream, $s_{k_m}$, at \gls{leo} \gls{lu}-$k_m$ respectively write as
	\begin{subequations}
		\begin{align}
			 & A_{subc,k_m}=S_{l,ck_m}^\prime+S_{l,pk_m}^\prime+{I_{l,k_m}^{tot}}^\prime+\sigma_n^2, \\
			 & B_{subc,k_m}=S_{l,pk_m}^\prime+{I_{l,k_m}^{tot}}^\prime+\sigma_n^2,                   \\
			 & A_{k_m}=S_{l,pk_m}^\prime+{I_{l,k_m}^{tot}}^\prime+\sigma_n^2,                        \\
			 & B_{k_m}={I_{l,k_m}^{tot}}^\prime+\sigma_n^2.
		\end{align}
	\end{subequations}

\end{appendices}
